# Supplementary material for: LMSeg: Unleashing the Power of Large-Scale Models for Open-Vocabulary Semantic Segmentation
Source: arXiv:2412.00364 source file (2026-02-18)
Supplement: Supplementary file 1 [file X_suppl.tex]

\clearpage
\maketitlesupplementary

% \section{The Use of Large Language Models (LLMs)}
% In this paper, we propose a novel approach that leverages Large Language Models (GPT-4) to generate attribute-enriched text prompts, enabling more precise alignment between visual and textual representations and achieving significant improvements in open-vocabulary semantic segmentation (OVSS). Specifically, we first generate candidate attributes and systematically validate their effectiveness through extensive experiments. Based on these results, we then select the optimal attribute combinations. Ultimately, this process yields the most effective text prompts for guiding OVSS.
%  \vspace{-2mm} 
\section{Ablation study on different LLMs}
Table~\ref{tab4_} reports the ablation results comparing different large language models used for generating attribute-enriched descriptions. We evaluate two representative LLMs: Qwen2.5~\cite{bai2025qwen2} and GPT-4~\cite{gpt} under six benchmarks. 
Across all datasets, GPT consistently outperforms Qwen, achieving higher mIoU on both large-scale (A-847, PC-459) and small-scale (A-150, PC-59) benchmarks. Notably, GPT also yields competitive or superior performance on VOC and VOCb. These results indicate that higher-quality language descriptions generated by stronger LLMs can further enhance the semantic alignment between visual and textual features, thereby improving segmentation performance.
\begin{table}[h]
    % \vspace{-2mm} 
    \centering
    % --- 表格 1 ---
    
    % \setlength{\tabcolsep}{0.2mm}
    \resizebox{1\linewidth}{!}{
    % \small 
    \begin{tabular}{c|c|c|c|c|c|c} \hline
    \toprule
    Methods & A-847 & PC-459 & A-150 & PC-59 & VOC & VOCb  \\ \hline
    Qwen2.5 & 12.4 & 19.6 & 32.1 & 58.4 & \textbf{96.0} & 79.7 \\
    GPT-4 & \textbf{13.1} & \textbf{20.3} & \textbf{33.3} & \textbf{59.7} & 95.4 & \textbf{81.1} \\
     \bottomrule
    \end{tabular}}
    \vspace{-2mm}
    % \captionsetup{width=0.95\linewidth}
    \caption{\textbf{Ablation study on different LLMs.} 
We conduct an ablation study to verify the effectiveness of different LLMs.} \label{tab4_}
\end{table}
 % \vspace{-10mm} 
\section{Ablation study on fine-tuning the encoder of LSMSeg.} 
Table~\ref{tab6} presents an ablation study on fine-tuning components of CLIP~\cite{clip}.
Due to computational cost constraints, the study did not fine-tune the SAM~\cite{sam} model, focusing instead on the specified CLIP components.
When we freeze the CLIP encoder, the lowest result is achieved across six datasets. 
The best fine-tuning strategy for CLIP is to fine-tune query and value projections only, with an average result of 50.5\%.
\begin{table}[h]
\centering
\resizebox{0.48\textwidth}{!}{
% \renewcommand\arraystretch{0.5}
% {
\small
\begin{tabular}{c|c|c|c|c|c|c|c} \hline
\toprule
Methods  & A-847 & PC-459 & A-150 & PC-59 & VOC & VOCb & avg. \\ \hline
Freeze & 8.1 & 13.3 & 25.9 & 46.9 & 83.4 & 61.6 & 39.9\\
CLIP$_{qk}$ & 11.6 & 18.2 & 30.7 & 56.2 & 94.7 & 78.5 & 48.3\\
CLIP$_{kv}$  & 12.7 & 19.9 & 32.8 & 59.0 & 95.0 &  80.2& 49.9\\
\rowcolor{darkgray!20}
CLIP$_{qv}$ & 13.1 & 20.3 & 33.2 & 59.7 & 95.4 & 81.1 &  50.5\\
\bottomrule
\end{tabular}
}
% \vspace{-2mm}
\caption{\textbf{Ablation study on fine-tuning the encoder of LSMSeg.} We conduct an ablation study on fine-tuning the CLIP encoder during training. $q,k$, and $v$ of CLIP are query, key, and value projections.} \label{tab6}
\end{table}
 % \vspace{-20mm} 
\section{Examples of Attribute-Enriched Text Descriptions}
In this section, we present some examples of detailed class descriptions generated using the GPT-4 model.

\vspace{2mm} 
\noindent \textbf{Generated descriptions for `bicycle'}
\begin{itemize}
    \item \texttt{A bicycle has a two-wheeled frame with handlebars and a seat, is medium-sized at around 1 to 1.5 meters in length, has a smooth metal frame, rubber tires, and textured handle grips, and is often red, blue, black, or metallic with shiny or matte finishes.}
\end{itemize}
\vspace{2mm} 
\noindent \textbf{Generated descriptions for `car'}
\begin{itemize}
    \item \texttt{A car has a boxy or sleek aerodynamic shape with four wheels, varies in size from compact to SUVs and large sedans, has a smooth metal body, rubber tires, and leather or fabric seats, and is usually white, black, red, or blue with a glossy finish.}
\end{itemize}
\vspace{2mm} 
\noindent \textbf{Generated descriptions for `airplane'}
\begin{itemize}
    \item \texttt{An airplane has a long fuselage with two wings and a tail fin, is very large, ranging from small private jets to massive airliners, has a smooth metal surface with rivets and windows, and is typically white, gray, or silver, sometimes with colorful airline logos.}
\end{itemize}
\vspace{2mm} 
\noindent \textbf{Generated descriptions for `bench'}
\begin{itemize}
    \item \texttt{A bench has a long, rectangular seat with a flat or slightly curved surface, is medium to large, seating two to four people, has a smooth wooden surface or a textured metal or stone finish, and is often brown, gray, or green, blending into outdoor environments.}
\end{itemize}

\subsection{More Qualitative Results}
We show more qualitative comparisons on PC-459 and ADE-150 in Figure~\ref{fig:vis2} and ~\ref{fig:vis3}.
\begin{figure*}[t]
    \centering
    % 第一行图片
    \begin{subfigure}[b]{0.24\textwidth}
        \centering
        \includegraphics[width=4.2cm,height=3.2cm]{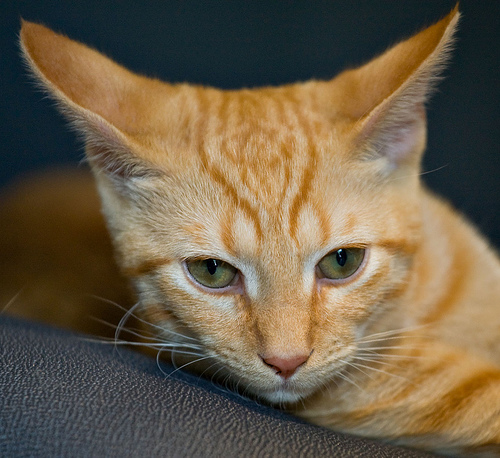}
        \includegraphics[width=4.2cm,height=3.2cm]{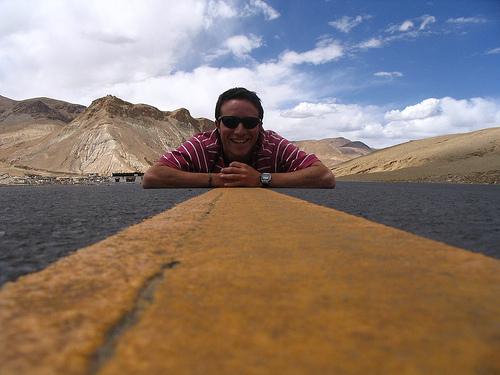}
         \includegraphics[width=4.2cm,height=3.2cm]{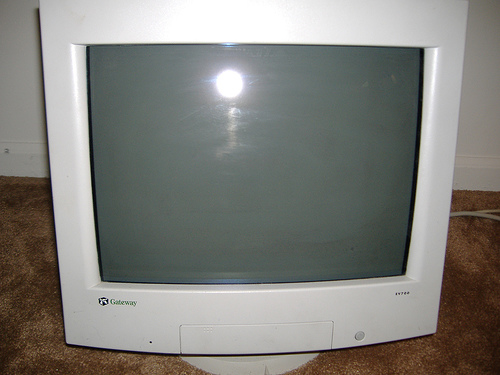}
        \caption{Image}
        % \label{fig:sub2}
    \end{subfigure}
    % \hspace{3mm} % 控制图片间的间隔
    \begin{subfigure}[b]{0.24\textwidth}
        \centering
        \includegraphics[width=4.2cm,height=3.2cm]{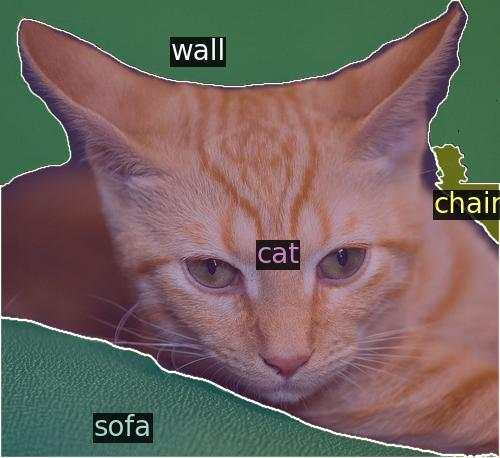}
       \includegraphics[width=4.2cm,height=3.2cm]{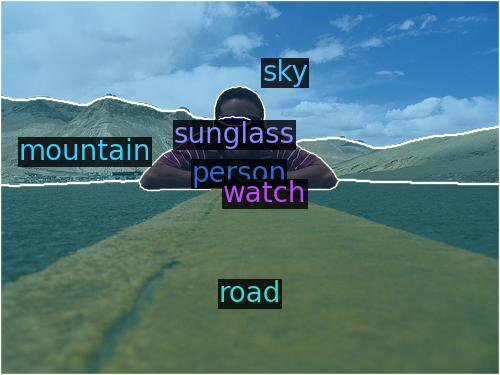}
         \includegraphics[width=4.2cm,height=3.2cm]{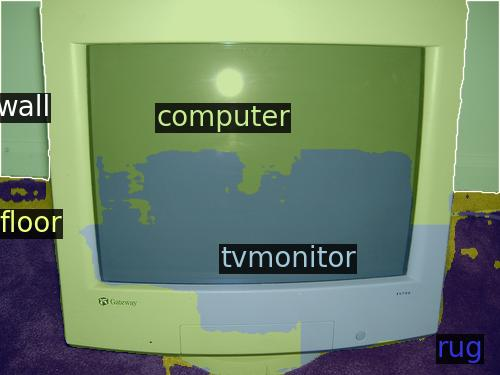}
        \caption{CAT-Seg}
        % \label{fig:sub2}
    \end{subfigure}
    % \hspace{3mm} % 控制图片间的间隔
    \begin{subfigure}[b]{0.24\textwidth}
        \centering
        \includegraphics[width=4.2cm,height=3.2cm]{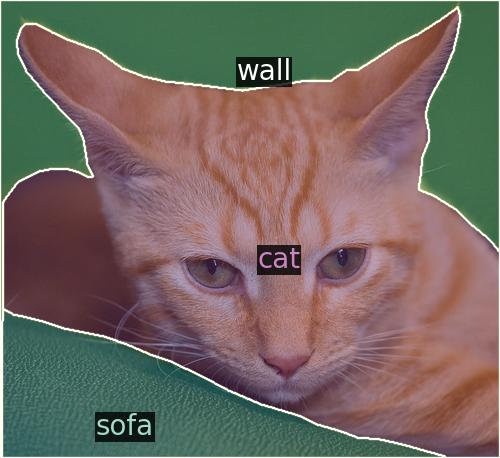}
        \includegraphics[width=4.2cm,height=3.2cm]{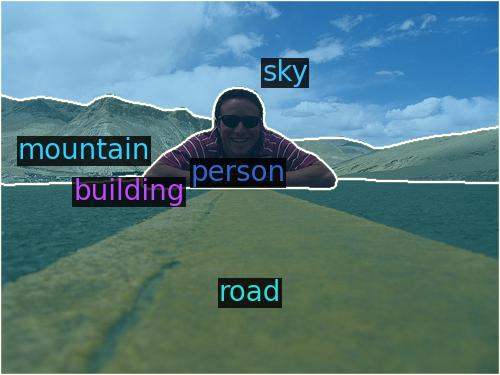}
         \includegraphics[width=4.2cm,height=3.2cm]{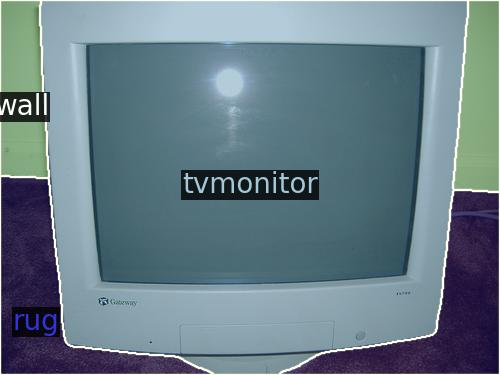} 
        \caption{LMSeg (ours)}
        % \label{fig:sub3}
    \end{subfigure}
    % \hspace{3mm} % 控制图片间的间隔
    \begin{subfigure}[b]{0.24\textwidth}
        \centering
        \includegraphics[width=4.2cm,height=3.2cm]{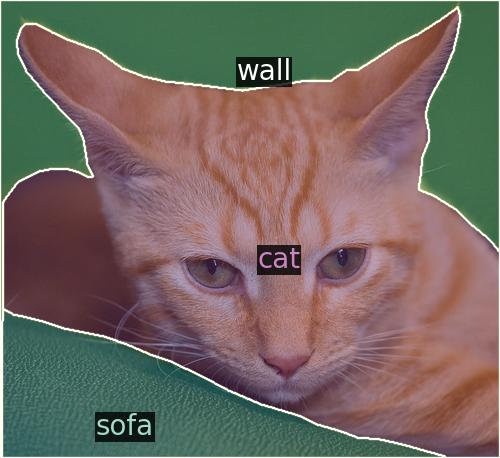}
        \includegraphics[width=4.2cm,height=3.2cm]{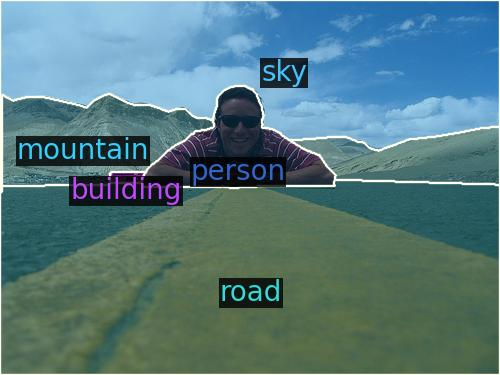}
         \includegraphics[width=4.2cm,height=3.2cm]{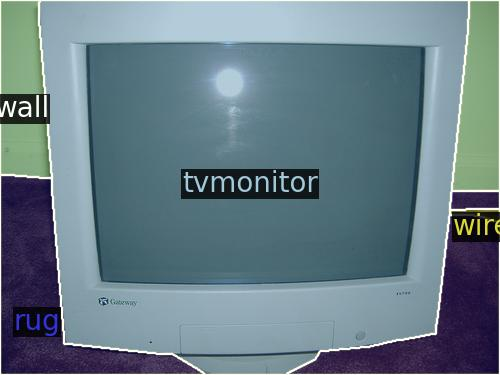}
        \caption{Ground truth}
        % \label{fig:sub4}
    \end{subfigure}
    \vspace{-2mm}
    \caption{\textbf{Qualitative comparisons on PC-459.}
     From left to right: input images, results of CAT-Seg, results of our LMSeg, and ground truth.}
    \label{fig:vis2}
\end{figure*}

\begin{figure*}[t]
    \centering
    % 第一行图片
    \begin{subfigure}[b]{0.24\textwidth}
        \centering
        \includegraphics[width=4.2cm,height=3.2cm]{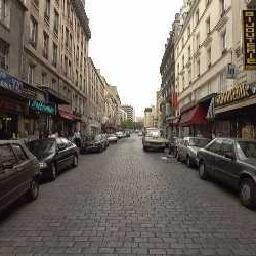}
        \includegraphics[width=4.2cm,height=3.2cm]{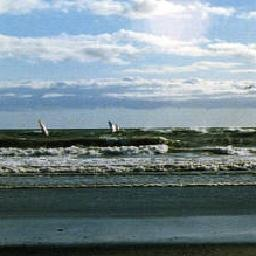}
        \includegraphics[width=4.2cm,height=3.2cm]{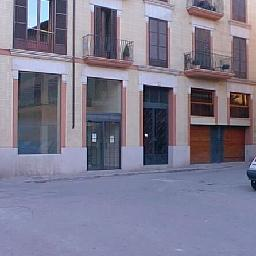}
        \caption{Image}
        % \label{fig:sub2}
    \end{subfigure}
    % \hspace{3mm} % 控制图片间的间隔
    \begin{subfigure}[b]{0.24\textwidth}
        \centering
        \includegraphics[width=4.2cm,height=3.2cm]{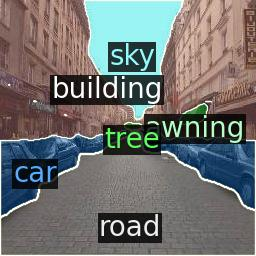}
        \includegraphics[width=4.2cm,height=3.2cm]{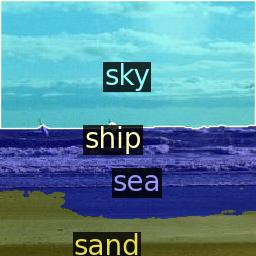}
        \includegraphics[width=4.2cm,height=3.2cm]{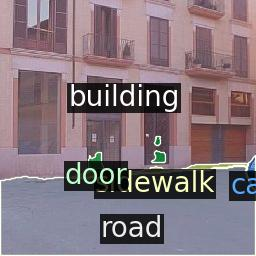}
        \caption{CAT-Seg}
        % \label{fig:sub2}
    \end{subfigure}
    % \hspace{3mm} % 控制图片间的间隔
    \begin{subfigure}[b]{0.24\textwidth}
        \centering
        \includegraphics[width=4.2cm,height=3.2cm]{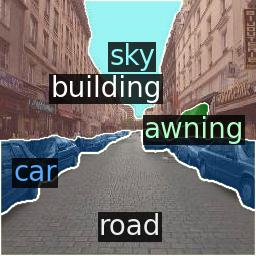}
        \includegraphics[width=4.2cm,height=3.2cm]{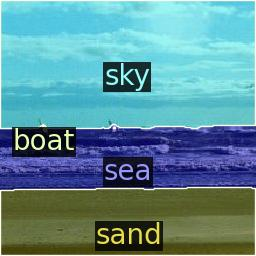}
        \includegraphics[width=4.2cm,height=3.2cm]{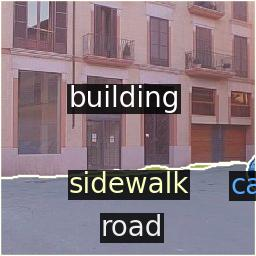}
        \caption{LMSeg (ours)}
        % \label{fig:sub3}
    \end{subfigure}
    % \hspace{3mm} % 控制图片间的间隔
    \begin{subfigure}[b]{0.24\textwidth}
        \centering
        \includegraphics[width=4.2cm,height=3.2cm]{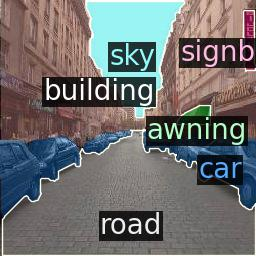}
        \includegraphics[width=4.2cm,height=3.2cm]{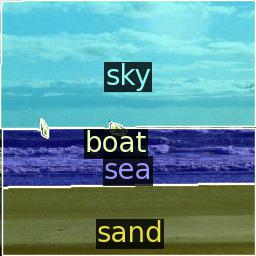}
        \includegraphics[width=4.2cm,height=3.2cm]{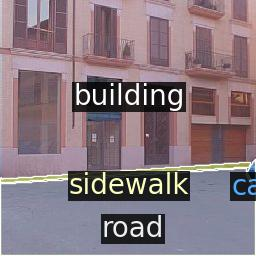}
        \caption{Ground truth}
        % \label{fig:sub4}
    \end{subfigure}
    \vspace{-2mm}
    \caption{\textbf{Qualitative comparisons on A-150.}
    From left to right: input images, results of CAT-Seg, results of our LMSeg, and ground truth.}
    \label{fig:vis3}
\end{figure*}
